# Supplementary material for: Magnon-polaron control in a surface magnetoacoustic wave resonator
Source: arXiv:2506.09717 ancillary file (2025-06-11)
Supplement: Supplementary file 1 [file supplement.pdf]

# Supplementary Information: Magnon-polaron control in a surface magnetoacoustic wave resonator

Kevin Künstle,[1,*] Yannik Kunz,[1] Tarek Moussa,[1] Katharina Lasinger,[1,2] Kei Yamamoto,[3] Philipp Pirro,[1] John F. Gregg,[2] Akashdeep Kamra,[1] and Mathias Weiler[1]

[1] *Fachbereich Physik and Landesforschungszentrum OPTIMAS, Rheinland-Pfälzische Technische Universität Kaiserslautern-Landau, 67663 Kaiserslautern, Germany*

[2] *Clarendon Laboratory, Department of Physics, University of Oxford, Parks Road, Oxford, OX1 3PU, United Kingdom*

[3] *Advanced Science Research Center, Japan Atomic Energy Agency, Tokai 319-1195, Japan*

## Supplementary Note 1: Resonator characteristics

The one-port surface acoustic wave (SAW) resonator employed in this study features a reflection-mitigating double-electrode interdigital transducer (IDT) centrally positioned between two Bragg mirrors, which function as reflective gratings for the acoustic waves. The double-electrode geometry of the IDT is implemented to suppress internal acoustic reflections, which can interfere with the establishment of a coherent standing wave within the planar resonator cavity. Each Bragg mirror comprises $N_\mathrm{g} = 100$ reflector stripes with a uniform finger width and spacing of 500 nm. The IDT exhibits an effective finger number $N_\mathrm{IDT}$ of 41, where each effective finger consists of two spatially separated fingers (250 nm width and spacing) connected to the same electrical contact. This geometry facilitates the excitation and resonant enhancement of a SAW with a wavelength of 2 µm.

### A: SAW Wavelength measurement using Brillouin Light scattering

The excited wavelength can directly be accessed using microfocussed Brillouin light scattering ($\mu$BLS) spectroscopy [1]. The $\mu$BLS signal intensity ($I_\mathrm{BLS}$) is proportional to the time averaged absolute value of the out-of-plane displacement $|u_\mathrm{z}|$ [2]:

$$I_\mathrm{BLS}(x) \propto \int_{T_0} |u_\mathrm{z}|^2 \,\mathrm{d}t \propto \sin^2(kx) \ . \tag{1}$$

Assuming a simplified standing wave $u_\mathrm{z}(x,t) = u_{\mathrm{z},0}\sin(kx)\sin(\omega t)$, the intensity is proportional to $\sin^2(kx)$. Here, $u_{\mathrm{z},0}$ denotes the amplitude, $k$ the wavenumber and $\omega$ the angular frequency. To determine the wave length of the excited standing wave, the $\mu$BLS laser spot was positioned between the mirror and the IDT. A 25 $\mu$m long linescan with a stepsize of 130 nm between mirror and IDT was conducted (x-direction). A microwave frequency exciting the central high-$Q$ mode of the resonator was applied and the resulting data is presented in Supplementary Fig. 1.

* kuenstle@rptu.de

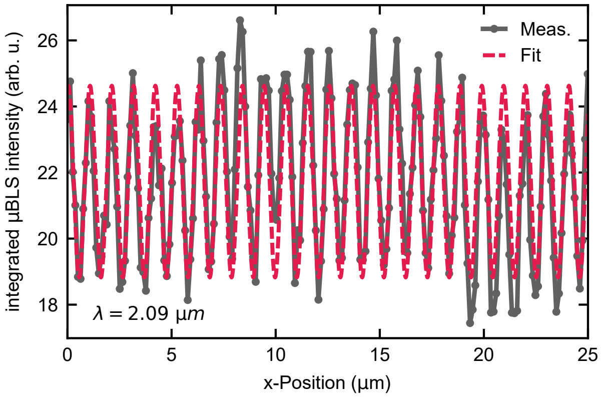


**Supplementary Fig.** 1: Measured integrated $\mu$BLS intensity over x-Position. Expected $\sin^2$ behavior is observed, from which a wavelength of $\lambda = 2.09\,\mu\text{m}$ is determined.

By fitting the data to a function of the form $I(x) = A\sin^2(kx + \theta) + B$, the wave length was determined to be $\lambda = 2.09\,\mu\text{m}$, which agrees well with the expected wavelength of $2\,\mu\text{m}$ theoretically supported by the resonator's geometry. The observed variations in peak height can be attributed to several factors, including changes in reflection depending on the laser spot position on the ZnO surface. Additionally, the laser spot has a diameter of approximately 300 nm, depending on the focus position, and follows a Gaussian profile. This implies that the measured intensity is averaged over a region approximately one-sixth of the wavelength. Consequently, the intensity does not completely drop to zero, resulting in a constant offset.

## B: SAW group velocity measurement using Brillouin Light scattering

To determine the group velocity ($v_{\text{gSAW}}$) of the excited surface acoustic wave, a time-resolved $\mu$BLS measurement was performed at a fixed frequency of 1.4 GHz. In this experiment, a short SAW pulse was generated at a specific time using an IDT distinct from the resonator structures. As the $\mu$BLS laser spot was incrementally positioned at increasing distances from this excitation IDT, the arrival time of the detected SAW pulse exhibited a corresponding shift due to the increased propagation path. The temporal profile of the detected SAW pulses was analyzed by fitting a sigmoidal Boltzmann function:

$$I_{\text{BLS}}(t) = C + \frac{A - C}{1 + e^{-\frac{t-t_0}{B}}}\ , \tag{2}$$

where the time delay parameter $t_0$, representing the arrival time of the pulse leading edge at the laser spot, was extracted for each spatial position. Subsequently, a linear fit was applied to the extracted $t_0$ values as a function of the distance between the excitation IDT and the laser spot. The slope of this linear fit directly yields the group velocity of the SAW. A detailed description of this procedure can be found in Supplementary Ref. [3]. The group velocity determined through this method was found to be $v_{\text{BLS}} = (2382.09 \pm 2.57)\,\text{m}\,\text{s}^{-1}$. The experimental data illustrating this measurement is presented in Supplementary Fig. 2, which displays the integrated $\mu$BLS intensity of the measured SAW pulses as a function of both the distance from the sending IDT to the laser spot and time. The dashed red line overlaid on the figure represents the linear fit applied to the inflection points of the Boltzmann fits (Supplementary Eq. (2)) for each spatial position.

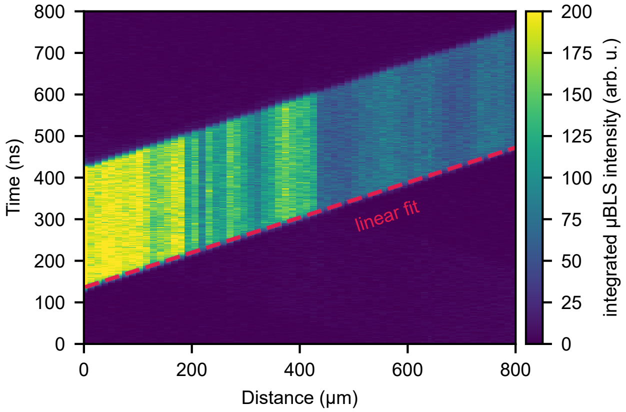


**Supplementary Fig.** 2: Integrated $\mu$BLS intensity in dependence of time and laser spot distance from the sending IDT. A SAW pulse is excited and detected at the position of the laser spot. By fitting the pulse flanks, the group velocity of the excited SAW was determined.

## C: Evaluated resonator properties

From the electrical measurement presented in the main text [Fig. 2d)], combined with the $\mu$BLS measurements shown above, further resonator properties can be accessed. Having three high-Q modes within the first resonator stopband, which represent well-defined cavity resonances, we can determine the free spectral range ($FSR$) of these resonances. Knowing the geometric parameters of the mirror electrode width $a = 500\,\mathrm{nm}$ and the distance between mirrors $d = 302\,\mu\mathrm{m}$, the reflection per single electrode in the mirror ($r_\mathrm{s}$) is calculated via [4]:

$$r_\mathrm{s} = \frac{2a}{\frac{v_\mathrm{gSAW}}{FSR} - d} = 2.01\,\% \ . \tag{3}$$

Knowing $r_\mathrm{s}$, the effective penetration depth into the mirrors ($L_\mathrm{p}$) can now be evaluated via [5]:

$$L_\mathrm{p} = \frac{\tanh[(N_\mathrm{g} - 1)r_\mathrm{s}]a}{r_\mathrm{s}} = 24.91\,\mu\mathrm{m} \ . \tag{4}$$

From these quantities, the effective resonator length $L_\mathrm{eff} = d + 2L_\mathrm{p}$ is found to be $L_\mathrm{eff} = 351.82\,\mu\mathrm{m}$. This quantity allows us to calculate the group velocity from the time domain data presented in the main text [Fig. 4c)]. Further, it is now possible to determine an effective quality factor of the resonator mirrors ($Q_\mathrm{g}$) [4]:

$$Q_\mathrm{g} = \frac{\pi(d + 2L_\mathrm{p})}{\lambda_\mathrm{SAW}[1 - \tanh(r_\mathrm{s}N_\mathrm{g})]} \ . \tag{5}$$

Here, $\lambda_\mathrm{p}$ denotes the acoustic wavelength.

Due to the external quality factor being significantly larger than the internal quality factor $Q_\mathrm{i}$, the total $Q$ factor is dominated by $Q_\mathrm{i}$, which can be separated into contributions from losses in the mirrors and propagation losses [4]:

$$\frac{1}{Q_\mathrm{i}} = \frac{1}{Q_\mathrm{g}} + \frac{v_\mathrm{gSAW}}{\pi \cdot f \cdot l_\mathrm{SAW}} \ . \tag{6}$$

In this equation $f$ denotes the frequency of the supported mode and $l_\mathrm{p}$ denotes the SAW decay length. It is now possible to calculate the decay length from the previously established parameters: $l_\mathrm{p} = 730.47\,\mu\mathrm{m}$, which agrees well with the one found by evaluating the time domain data as seen in Supplementary Note 1D (757 µm).

### D: Resonator in time domain

Following the approach detailed in the main text methods section, the frequency domain data of the resonator can be transformed into the time domain. Here, we demonstrate how information extracted from this time-domain transformation can be used to further characterize the resonator properties. Therefore, Supplementary Fig. 3 displays the off-resonant blue line cut presented in Fig. 4f) of the main text. Each peak visible corresponds to the SAW passing the IDT which is located in the center of the resonator. Knowing the effective resonator length $L_{\mathrm{eff}}$, we can now calculate the SAW group velocity and the decay length. These values can then be compared to those obtained through other evaluation methods.

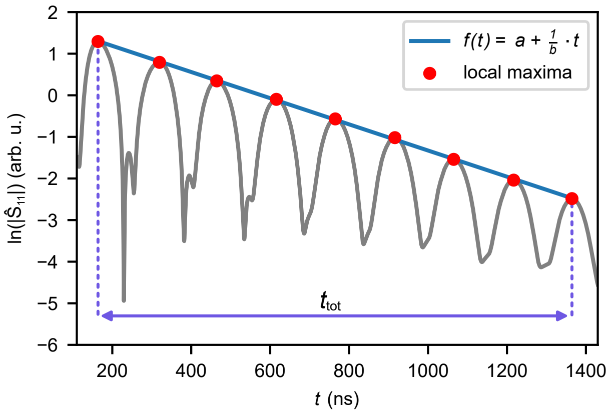


**Supplementary Fig.** 3: Natural logarithm of the time domain $|\hat{S}_{11}|$ reflection parameter in dependence of time $t$. The local maxima marked by the red points identify the single passes of the SAW through the resonator. By fitting a linear function to these maxima (blue line) the exponential decay $(1/b)$ is accessed. Further, $t_{\mathrm{tot}}$ marks the time the SAW takes to pass the resonator 8 times.

To better visualize the exponential nature of the SAW decay, the natural logarithm of the $|\hat{S}_{11}|$ data is shown in Supplementary Fig. 3. To find the decay length, the local maxima (red dots) are fitted using the linear function $f(t) = a + (1/b) \cdot t$, where $a$ is the y-axis offset and $1/b$ represents the exponential decay constant. Knowing the SAW group velocity presented in Note 1B ($v_{\mathrm{BLS}} = 2382\,\mathrm{m\,s^{-1}}$), the decay length is calculated via $l_{\mathrm{SAW}} = b \cdot v_{\mathrm{BLS}} = 757\,\mu\mathrm{m}$. This value agrees well with the previously calculated decay length of $730\,\mu\mathrm{m}$.

In Supplementary Fig. 3, $t_{\mathrm{tot}}$ denotes the total time taken for the SAW to complete eight passes through the resonator. The group velocity is now calculated via $v_{\mathrm{gSAW}} = \frac{8 \cdot L_{\mathrm{eff}}}{t_{\mathrm{tot}}} = 2344\,\mathrm{m\,s^{-1}}$, which is again in agreement with the directly accessed group velocity employing timeresolved $\mu$BLS spectroscopy of $2382\,\mathrm{m\,s^{-1}}$.

The strong consistency between the results obtained from various, distinct evaluation methods presented in Supplementary Note 1 underscores a comprehensive understanding of our SAW resonator's behavior.

## Supplementary Note 2: Broad band FMR and VSM measurements

To find the saturation magnetization $M_{\mathrm{s}}$, a vibrating sample magnetometer measurement was conducted on a reference YIG chip from the same wafer, utilizing the Physical Property Measurement System (PPMS) by Quantum Design. A hysteresis loop at room temperature was recorded, resulting in a saturation magnetization of $M_{\mathrm{s}} = 127\,\mathrm{kA\,m^{-1}}$, which is in reasonable agreement with literature values around $140\,\mathrm{kA\,m^{-1}}$. Broadband ferromagnetic resonance spectroscopy was subsequently performed to find the crystal anisotropy field $M_{\mathrm{ani}}$ and the g-factor. However, for YIG films that are no longer thin films, many PSSW modes arise very close to the FMR frequency. This can be seen in Supplementary Fig. 4a), where the magnetic field derivative of the real part of the transmission parameter $S_{21}$ is color-coded as a function of frequency and magnetic field [6]. From the lowest frequency signal visible as a function of field, the resonance positions are extracted and subsequently fitted to the Kittel equation [7]:

$$f = \frac{g\mu_{\mathrm{B}}}{h}\sqrt{(\mu_0 H_{\mathrm{res}} + \mu_0 H_{\mathrm{ani}}) \cdot (\mu_0 H_{\mathrm{res}} + \mu_0 H_{\mathrm{ani}} + \mu_0 M_{\mathrm{s}})}\ , \tag{7}$$

where $f$ denotes the frequency, $H_{\mathrm{res}}$ the found resonance field, and $h$ Planck's constant. The found $g$-factor is $g = 2.18$, and the anisotropy field is small, as expected: $\mu_0 H_{\mathrm{ani}} = 0.99\,\mathrm{mT}$. Due to the presence of numerous

other magnetic excitations near the FMR frequency, the extracted $g$-factor and anisotropy field should be considered approximate. A linecut at a fixed magnetic field is shown in Supplementary Fig. 4c), where clearly many magnetic excitations are visible. These excitations are compared to the first 10 calculated PSSW modes with an in-plane $k$-number of 0, as depicted on top of the measurement data in Supplementary Fig. 4b). The calculations agree well with the measured excitations and show that this behavior is predicted.

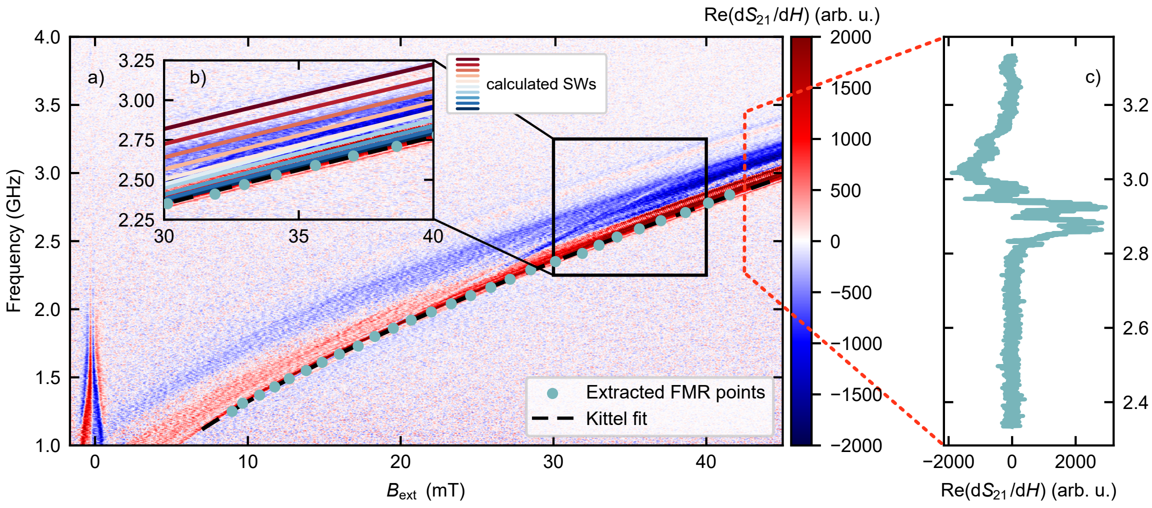


**Supplementary Fig.** 4: a) Broadband FMR measurement of YIG/ZnO sample. The lowest frequency mode exhibiting a clear field dependence represents the FMR and is used to characterize resonance positions. Kittel fit is shown as a black dashed line. b) First 10 calculated SW modes with an in-plane k-number of 0, depicted on top of the measurement data. Calculated modes agree well with the measured excitations. c) Signal at a fixed magnetic field showing a multitude of magnetic excitations.

## Supplementary Note 3: Direct SW excitation and SW loss rate evaluation

As discussed in main text Sec. 2.1 , the spin wave (SW) loss rate is extracted from the direct SW excitation located in the center of the anticrossing. This direct excitation is attributed to a spurious RF current present in the microstructures [8]. A depiction of the central high-$Q$ mode at 0° is shown in Supplementary Fig. 5a). The direct excitation is visible as the line centered in the anticrossing. This direct excitation also exhibits a smaller anticrossing feature, highlighted by the red dashed ellipse. To obtain the SW loss rate $\kappa_{\mathrm{m}}$, the frequency linewidth of the direct excitation is extracted by fitting a Lorentzian to the linecut shown by the dashed red line. The fit and cut are shown in Supplementary Fig. 5b). Here, we find a loss rate of $\kappa_{\mathrm{m}}/2\pi = (1.24 \pm 0.02)\,\mathrm{MHz}$. To determine $\kappa_{\mathrm{m}}$ for other angles, we employed the approach outlined in Supplementary Ref. [9]. This method utilizes a simplified version of the Kalinikos-Slavin spin wave dispersion relation, from which the following expression for the angular frequency linewidth ($\Delta\omega$) is derived:

$$\Delta\omega = \alpha\sqrt{\left(\frac{1}{2}\gamma\mu_0(H_{\mathrm{x}}^{\mathrm{dip}} - H_{\mathrm{y}}^{\mathrm{dip}})\right)^2 + \omega^2}, \tag{8}$$

where $\omega$ is the angular frequency of the SW mode. The contributing fields $H_{\mathrm{x}}^{\mathrm{dip}}$ and $H_{\mathrm{y}}^{\mathrm{dip}}$ are given by:

$$H_{\mathrm{x}}^{\mathrm{dip}} = M_{\mathrm{s}}\frac{1-e^{-kd}}{kd}, \quad H_{y}^{\mathrm{dip}} = M_{\mathrm{s}}\left(1 - \frac{1-e^{-kd}}{kd}\right)\sin^2\phi\ . \tag{9}$$

In these Supplementary equations, $M_{\mathrm{s}}$ denotes the saturation magnetization, $k$ the in-plane wavenumber, $d$ the film thickness, $\phi$ the angle between the external field and the magnetization direction, and $\alpha$ denotes the Gilbert damping. At the fixed angle of 0°, where all parameters in Supplementary Eq. (8) are known except for $\alpha$, we solved for $\alpha$, yielding $\alpha = 9 \times 10^{-4}$, which is in the right order of magnitude for YIG.

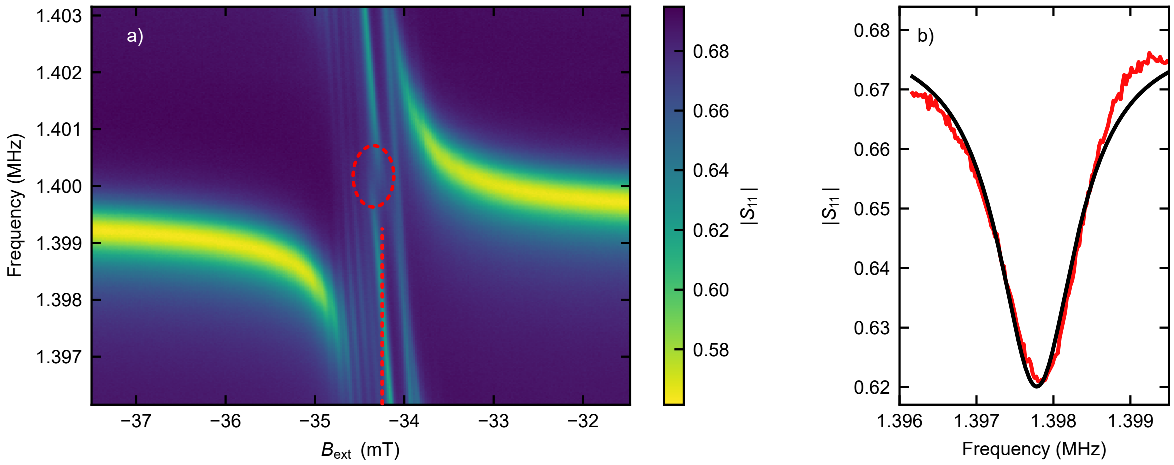


**Supplementary Fig.** 5: a) Anticrossing with fundamental SW excitation at 0° of central high-$Q$ mode. Central line corresponds to direct SW excitation, exhibiting a secondary anticrossing (red dashed ellipse). Dashed red line marks the linecut used to evaluate the loss rate. b) Red line depicts the extracted linecut from a). It is fitted with a Lorentzian function (black) to extract the SW loss rate.

## Supplementary Note 4: Angle dependent SW velocity

Our system enables coupling to magnons with a non-zero group velocity. To determine this velocity, we calculated the derivative of the spin wave angular frequency $\omega$ with respect to the wave vector $k$, $\mathrm{d}\omega/\mathrm{d}k$, derived from the general Kalinikos-Slavin dispersion relation. For each measured angle, this dispersion relation was evaluated at a fixed magnetic field corresponding to the observed anticrossing ($B_{\mathrm{ac}}$). The spin wave group velocity ($v_{\mathrm{gSW}}$) was then obtained by evaluating this derivative at the wave vector of the SAW. The calculated velocities are presented in Supplementary Fig. 6, which clearly shows that the maximum coupling observed at 0°, for instance, occurs at an angle where the SW group velocity is indeed non-zero.

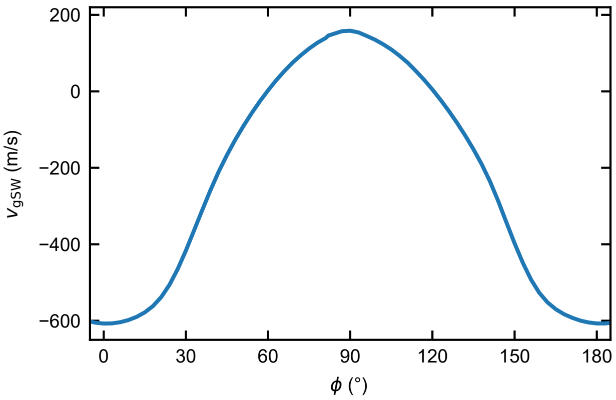


**Supplementary Fig.** 6: Spin wave group velocity $v_{\mathrm{gSW}}$ as a function of magnetic field direction $\phi$.

## Supplementary Note 5: Angle dependent coupling strength of all SW evaluated modes

Complementing the $n = 0$ mode presented in main text Fig. 3g), Supplementary Fig. 7 displays the coupling strength as a function of the angle $\phi$ (between the external magnetic field and the SAW wave vector) for all evaluated spin wave modes. The coupling strength $g$ exhibits distinct qualitative and quantitative angular dependencies for different

SW modes. This behavior is attributed to the varying degree of mode overlap between the spin wave and surface acoustic wave profiles as the angle changes.

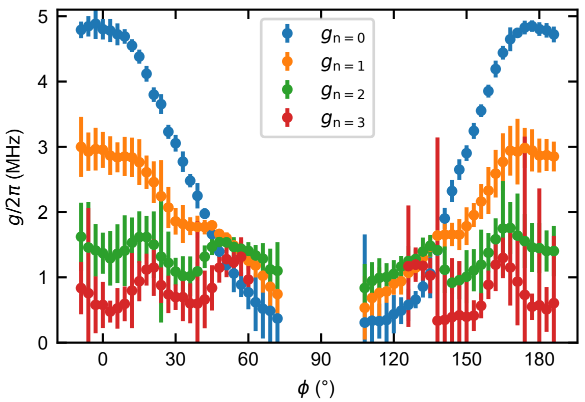


**Supplementary Fig.** 7: Coupling strength of the evaluated SW modes with respect to external field direction $\phi$.

## Supplementary Note 6: Simple model of Rabi-like oscillations

As discussed in main text Sec. 2.3, the Rabi frequency of the coupled magnon-phonon system can be calculated from the detuning $\delta$ and the coupling strength $g$, both accessible through frequency domain analysis. Following the standard approach for two-level systems [10], the probability $P_\mathrm{m}(t)$ of finding the system in the uncoupled magnon eigenstate at time $t$ is given by Rabi's formula:

$$P_\mathrm{m}(t) = \frac{4g^2}{\omega_\mathrm{rabi}^2} \sin^2\left(\frac{\omega_\mathrm{rabi}}{2} t\right) \ , \tag{10}$$

where $\omega_\mathrm{rabi}$ is the angular Rabi frequency, defined as:

$$\omega_\mathrm{rabi} = \sqrt{4g^2 + \delta^2} \ , \text{with} \quad \delta = \gamma |B_\mathrm{ac} - B_\mathrm{ext}| \ . \tag{11}$$

Here, the $\delta$ is determined by the linear shift of the SW dispersion with the applied magnetic field in the vicinity of the anticrossing, as discussed in the main text. This field shift is quantified by the difference between the anticrossing field $B_\mathrm{ac}$ and the external field $B_\mathrm{ext}$. The resulting theoretical calculation of $P_\mathrm{m}(t)$ as a function of time and magnetic field is presented in Supplementary Fig. 8. The characteristic hat-like shape, also observed in the time-domain experimental data, is clearly visible.

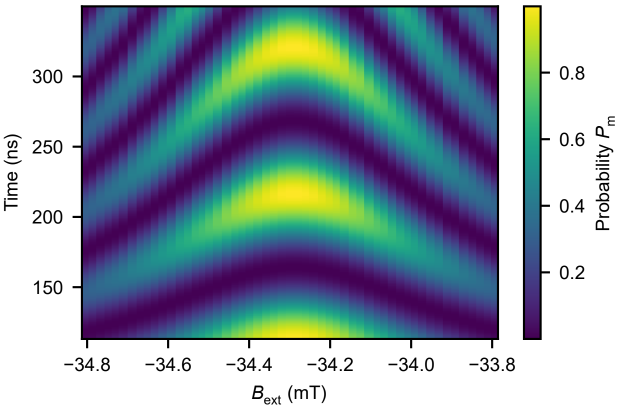


**Supplementary Fig.** 8: Rabi-like oscillations evaluated using the coupling strength $g$ and detuning $\delta$, accessed via frequency domain analysis. The characteristic hat-shaped probability to find the system in the magnon eigenstate $P_{\mathrm{m}}(t)$ is visible as a function of time and magnetic field (implied by the use of $\delta$).

It is important to note that this simplified two-level model does not fully capture the complexity of our experimental system. Specifically, it neglects the multiple SAW passes occurring concurrently within the resonator, as well as the influence of spurious signals and the directly excited spin wave mode observed at the anticrossing center (detailed in Supplementary Note 4). We present this simplified model solely to illustrate the characteristic hat-shaped behavior of the magnon population oscillations, which is qualitatively consistent with the time-domain data presented in the main text, despite these additional complexities.

## Supplementary Note 7: Theoretical description of magnon-phonon coupling

This section discusses in detail the theoretical framework describing the magnon–phonon coupling strength in our device. Due to the YIG film being 1.98 µm thick, the numerical tool TetraX [11, 12] is used to access the SW mode profiles in this film. For the simulations, a saturation magnetization of $M_{\mathrm{s}} = 127\,\mathrm{kA\,m^{-1}}$ was used, as determined by vibrating sample magnetometry measurements on a reference chip. The exchange stiffness was set to $A = 3.75 \times 10^{-12}\,\mathrm{J\,m^{-1}}$. The geometry was modeled as a single-layer film with a thickness of 1980 nm and a uniform mesh spacing of 5 nm. Mode profiles were extracted at a wave vector of $k = 3.02\,\mathrm{rad\,\mu m^{-1}}$, corresponding to the SAW wave vector in the resonator discussed in Supplementary Note 1B.

From previous work it is known, that the initially excited SAW modes in a similar material stack are Rayleigh-like surface acoustic waves [3], however they have a nonvanishing shear-displacement component which can be amplified by the SAW resonator. We therefore allow all displacement components to enter the calculation. These elastic displacements are assumed to decay exponentially from the surface. This classical description of elastic and magnetization dynamics is then quantized and expressed in terms of quasiparticles- phonons and magnons. Employing the ensuing relations, magnetoelastic energy is expressed in terms of a Hamiltonian involving phonons and magnons, which directly yields the magnon-phonon coupling strength. We largely follow the approach in Supplementary Ref. [13] correcting and generalizing it as per the requirements of our system.

### A: Outline of the quantization procedure

We introduce the relation between classical and quantum formalisms using the simple example of elastic displacements on a 1D string [14]. Consider the classical Hamiltonian:

$$H_{\mathrm{1D}} = \int_L \mathrm{d}x \left[\frac{1}{2}\rho\dot{u}^2 + \frac{1}{2}T\left(\frac{\partial u}{\partial x}\right)^2\right] \tag{12}$$

describing a one-dimensional elastic displacement $u$ on a string. Here, $\rho$ is the mass density, $T$ parametrizes the elastic potential energy, and $L$ is the string length. In order to obtain the eigenmode profiles and frequencies, one typically expresses the displacement in terms of orthonormal functions $\phi_k(x)$ that satisfy the boundary conditions imposed on

the system:

$$u(x) = \sum_k q_k \phi_k(x), \tag{13}$$

where $q_k$ parametrize the different contributions and $k$ labels the distinct orthonormal functions which satisfy the orthonormality condition:

$$\int_L dx\ \phi_k(x)\phi^*_{k'}(x) = \delta_{k,k'}. \tag{14}$$

With these substitutions, one can proceed towards bringing the classical Hamiltonian [Supplementary Eq. (12)] into a diagonal form in terms of the different $k$ modes. From this point on, one can quantize by identifying the canonical position and momentum, making them operators, and postulating the appropriate commutation relation between them. The procedure is described, for example, in Supplementary Ref. [14].

We pause to discuss the key points in this mathematical procedure. First, the orthonormal functions $\phi_k(x)$ that satisfy Supplementary Eq. (14) become the quasiparticle wavefunctions after the quantization procedure. Thus, within the quantum framework, their orthonormality ensures that the different quasiparticles do not interact (disregarding higher order nonlinearities) and that the probability of finding a single quasiparticle somewhere in all space is unity. Secondly, the commonly employed example of an infinite medium [14] is modeled via the periodic boundary conditions: $u(x+L) = u(x)$ which results in plane waves basis $\phi_k(x) = (1/\sqrt{L})\ \exp(ikx)$ with discrete values of $k$ imposed by the condition: $u(x+L) = u(x)$. In this manner, the boundary conditions are the key to determining the orthonormal basis functions irrespective of whether we use classical or quantum description. If one considered a finite medium and some confinement boundary conditions on the edges, the exact nature of the basis functions $\phi_k(x)$ depends on the precise boundary conditions.

## B: Quantization of the phonon and magnon modes

We first consider the elastic degrees of freedom with a coordinate system such that the wave vector is along x axis and the film out-of-plane direction is along the z axis. Furthermore, we consider the three-dimensional elastic displacement with components $u_{\rm x}\hat{x}$, $u_{\rm y}\hat{y}$, and $u_{\rm z}\hat{z}$. We consider a SAW which is confined by an acoustic resonator such that it forms a standing wave profile in the x direction and decays exponentially along z axis with the surface lying at $z = 0$. With these conditions and following the quantization procedure outlined in Sec. VII A, we may write the quantized expressions for the displacements:

$$\tilde{u}_{\rm x} = \sqrt{\frac{\hbar}{\rho A \omega_{\rm p}}} t_{\rm x} f(z) \sin(k_{\rm p} x + \phi_{\rm p})(\tilde{a} + \tilde{a}^\dagger), \tag{15}$$

$$\tilde{u}_{\rm y} = \sqrt{\frac{\hbar}{\rho A \omega_{\rm p}}} t_{\rm y} f(z) \sin(k_{\rm p} x + \phi_{\rm p})(\tilde{a} + \tilde{a}^\dagger), \tag{16}$$

$$\tilde{u}_{\rm z} = \sqrt{\frac{\hbar}{\rho A \omega_{\rm p}}} t_{\rm z} f(z) \sin(k_{\rm p} x + \phi_{\rm p})(\tilde{a} + \tilde{a}^\dagger), \tag{17}$$

where $\rho$ is the material density assumed to be spatially uniform for simplicity, $A$ is the area of confinement due to the acoustic resonator, $\omega_{\rm p}$ and $k_{\rm p}$ are the angular frequency and wavenumber of the phonon mode under consideration, $\tilde{a}$ is the annihilation operator for the phonon mode, $t_{\rm x,y,z}$ parametrize the relative strength of the displacement components and they follow the constraint $t_{\rm x}^2 + t_{\rm y}^2 + t_{\rm z}^2 = 1$, and $f(z)$ parametrizes the spatial dependence and decay of the mode. Here, $\phi_{\rm p}$ is the standing wave phase that depends on the precise boundary conditions. Due to the complex nature of our acoustic cavity, we are unable to fully ascertain $\phi_{\rm p}$ and assume it to be zero. We discuss this issue further below. In our simplified model, we assume $f(z)$ to be a simple exponential decay that follows the normalization condition:

$$\int_0^\infty dz |f(z)|^2 = 1, \tag{18}$$

$$\implies f(z) = \sqrt{\frac{2}{z_{\rm d}}} e^{-\frac{z}{z_{\rm d}}}, \tag{19}$$

where $z_{\rm d}$ parametrizes the decay length. Employing Supplementary Eqs. (15) - (17) with $\phi_{\rm p} = 0$, we obtain the expression for the relevant components of the strain tensor:

$$\tilde{e}_{\rm xx} = \frac{\partial \tilde{u}_{\rm x}}{\partial x} = k_{\rm p}\sqrt{\frac{\hbar}{\rho A \omega_{\rm p}}} t_{\rm x} f(z)\cos(k_{\rm p}x)(\tilde{a}+\tilde{a}^\dagger), \tag{20}$$

$$\tilde{e}_{\rm xz} = \frac{1}{2}\left(\frac{\partial \tilde{u}_{\rm x}}{\partial z} + \frac{\partial \tilde{u}_{\rm z}}{\partial x}\right), \tag{21}$$

$$= \frac{1}{2}\sqrt{\frac{\hbar}{\rho A \omega_{\rm p}}} t_{\rm x} f'(z)\sin(k_{\rm p}x)(\tilde{a}+\tilde{a}^\dagger)$$

$$+ \frac{k_{\rm p}}{2}\sqrt{\frac{\hbar}{\rho A \omega_{\rm p}}} t_{\rm z} f(z)\cos(k_{\rm p}x)(\tilde{a}+\tilde{a}^\dagger). \tag{22}$$

$$\tilde{e}_{\rm xy} = \frac{1}{2}\left(\frac{\partial \tilde{u}_{\rm x}}{\partial y} + \frac{\partial \tilde{u}_{\rm y}}{\partial x}\right), \tag{23}$$

$$= \frac{k_{\rm p}}{2}\sqrt{\frac{\hbar}{\rho A \omega_{\rm p}}} t_{\rm y} f(z)\cos(k_{\rm p}x)(\tilde{a}+\tilde{a}^\dagger), \tag{24}$$

$$\tilde{e}_{\rm yz} = \frac{1}{2}\left(\frac{\partial \tilde{u}_{\rm y}}{\partial z} + \frac{\partial \tilde{u}_{\rm z}}{\partial y}\right), \tag{25}$$

$$= \frac{1}{2}\sqrt{\frac{\hbar}{\rho A \omega_{\rm p}}} t_{\rm y} f'(z)\sin(k_{\rm p}x)(\tilde{a}+\tilde{a}^\dagger) \tag{26}$$

$$\tilde{e}_{\rm zz} = \frac{\partial \tilde{u}_{\rm z}}{\partial z} = \sqrt{\frac{\hbar}{\rho A \omega_{\rm p}}} t_{\rm z} f'(z)\sin(k_{\rm p}x)(\tilde{a}+\tilde{a}^\dagger). \tag{27}$$

The corresponding quantized expressions for the magnetization components in a coordinate system (see Supplementary Fig. 9) with $z'$ axis aligned with the equilibrium magnetization are obtained as [13, 15]:

$$\tilde{m}_{\rm x'} = \sqrt{\frac{\gamma\hbar M_{\rm s}}{A}}\cos(k_{\rm p}x+\phi_{\rm m})\mathcal{M}_{\rm ip}(z)\left(\tilde{c}+\tilde{c}^\dagger\right), \tag{28}$$

$$\tilde{m}_{\rm y'} = \frac{1}{i}\sqrt{\frac{\gamma\hbar M_{\rm s}}{A}}\cos(k_{\rm p}x+\phi_{\rm m})\mathcal{M}_{\rm oop}(z)\left(\tilde{c}^\dagger-\tilde{c}\right), \tag{29}$$

where $M_{\rm s}$ is the saturation magnetization, $\gamma$ is the gyromagnetic ratio magnitude, $\tilde{c}$ is the magnon annihilation operator, $\mathcal{M}_{\rm ip,oop}(z)$ capture the spatial profile and ellipticity of the magnetostatic mode which is frequency and wavenumber matched with the phonon mode. The spatial profile of the magnetostatic mode is evaluated numerically within the Landau-Lishitz framework and is considered an input to our analysis. Further, it obeys the normalization condition

$$\int_{FM} {\rm d}z\ \mathcal{M}_{\rm ip}(z)\mathcal{M}^*_{\rm oop}(z) = 1, \tag{30}$$

where the integration is over the ferromagnet (FM) thickness. When $\mathcal{M}_{\rm ip,oop}$ are available only for propagating modes, one should obtain the effective $\mathcal{M}_{\rm ip,oop}$ by averaging over the forward and backward propagating modes, and then normalize the resulting function using the Supplementary equation above. A more detailed quantization procedure can be found in Ref. [16, 17].

As in the case of phonons, $\phi_{\rm m}$ depends on the exact boundary conditions for the magnetization. There is an extra layer of complication here. One might expect the magnons to not be confined by the acoustic resonator at all. However, in the regime of interest to us, phonons and magnons hybridize and the acoustic boundary conditions affect and confine the hybrid quasiparticle. Taking this implicitly into account, in our considerations above, we have already assumed that the magnon is confined to the region defined by the acoustic resonator. This is yet another reason for our inability to rigorously account for the boundary conditions experienced by the hybrid quasiparticle. We again assume $\phi_{\rm m} = 0 = \phi_{\rm p}$ and that any error introduced by these assumptions does not affect the qualitative physics and dependencies.

### C: Magnetoelastic coupling to magnon-phonon coupling

We are now ready to consider the magnetoelastic energy, expressed classically in a cubic [100] system as

$$H_{\rm mec} = \int_{FM} {\rm d}^3r\; b_1 \left( \frac{m_{\rm x}^2}{M_{\rm s}^2} e_{\rm xx} + \frac{m_{\rm z}^2}{M_{\rm s}^2} e_{\rm zz} \right) + 2b_2 \left( \frac{m_{\rm x} m_{\rm z}}{M_{\rm s}^2} e_{\rm xz} + \frac{m_{\rm x} m_{\rm y}}{M_{\rm s}^2} e_{\rm xy} + \frac{m_{\rm y} m_{\rm z}}{M_{\rm s}^2} e_{\rm yz} \right), \tag{31}$$

where we have disregarded the term containing the vanishing strain component $e_{yy}$. Owing to the weak anisotropies in YIG and to maintain clarity and brevity in the theoretical treatment, the coordinate system used to express the magnetoelastic energy is not rotated into the [111] crystallographic frame of the employed YIG film. The magnetoelastic constants are denoted by $b_1 = 3.48 \times 10^5\,{\rm J\,m^{-3}}$ and $b_2 = 3.48 \times 10^5\,{\rm J\,m^{-3}}$ [18]. Assuming that an in-plane applied magnetic field saturates the equilibrium magnetic moment along $\hat{z}'$ (Supplementary Fig. 9), we obtain the following relation between the magnetization in the two coordinate frames:

$$m_{\rm x} = M_{\rm s} \cos\phi - m_{\rm x'} \sin\phi, \quad m_{\rm z} = m_{\rm y'}, \quad m_{\rm y} = M_{\rm s} \sin\phi + m_{\rm x'} \cos\phi, \tag{32}$$

where $m_{\rm x'}$ and $m_{\rm y'}$ are the small deviations characterizing the magnetization dynamics.

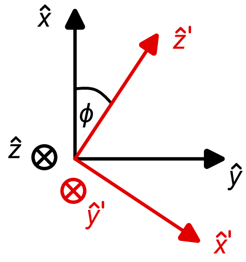


**Supplementary Fig.** 9: Schematic for the two coordinate systems. The primed coordinate system is used to characterize the magnetic ground state (magnetization pointing along $\hat{z}'$) and dynamics, while the unprimed coordinate system describes the lattice better. $\phi$ is thus the angle between the equilibrium magnetic moment and the wave vector direction $\hat{x}$.

Employing the transformations above in Supplementary Eq. (31) and retaining only the terms linear in the small variables $m_{x'}$ and $m_{y'}$, we obtain

$$H_{\rm mec} = \int_{FM} {\rm d}^3r\; 2b_2 \left( \cos\phi \frac{m_{\rm y'}}{M_{\rm s}} e_{\rm xz} + \cos(2\phi) \frac{m_{\rm x'}}{M_{\rm s}} e_{\rm xy} + \sin\phi \frac{m_{\rm y'}}{M_{\rm s}} e_{\rm yz} \right) - b_1 \sin(2\phi) \frac{m_{\rm x'}}{M_{\rm s}} e_{\rm xx}. \tag{33}$$

Employing Supplementary Eqs. (20)-(29) in Supplementary Eq. (33) above and making the rotating wave approximation (i.e., disregarding terms of the sort $\tilde{a}\tilde{c}$ and $\tilde{a}^\dagger \tilde{c}^\dagger$), we obtain the quantum Hamiltonian for magnon-phonon coupling:

$$\tilde{H}_{\rm mec} = -\hbar g_1 \left( \tilde{a}\tilde{c}^\dagger + \tilde{a}^\dagger \tilde{c} \right) - \hbar i g_2 \left( \tilde{a}\tilde{c}^\dagger - \tilde{a}^\dagger \tilde{c} \right), \tag{34}$$

where

$$g_1 = \frac{k_{\rm p}}{2} \sqrt{\frac{\gamma}{\rho \omega_{\rm p} M_{\rm s}}} \left[ b_1\; I_{\rm x,ip}(\phi)\; \sin(2\phi) - b_2\; I_{\rm y,ip}(\phi)\; \cos(2\phi) \right], \tag{35}$$

$$I_{\rm x,ip}(\phi) = \int_{FM} dz\; t_{\rm x} f(z) \mathcal{M}_{\rm ip}(z), \tag{36}$$

$$I_{\rm y,ip}(\phi) = \int_{FM} dz\; t_{\rm y} f(z) \mathcal{M}_{\rm ip}(z), \tag{37}$$

$$g_2 = \frac{k_{\rm p}}{2} \sqrt{\frac{\gamma}{\rho \omega_{\rm p} M_{\rm s}}}\; b_2\; I_{\rm z,oop}(\phi)\; \cos(\phi), \tag{38}$$

$$I_{\rm z,oop}(\phi) = \int_{FM} dz\; t_{\rm z} f(z) \mathcal{M}_{\rm oop}(z). \tag{39}$$

With these definitions, Supplementary Eq. (34) can be expressed as:

$$\tilde{H}_{\rm mec} = -\hbar \left(g \ \tilde{a}\tilde{c}^\dagger + g^* \ \tilde{a}^\dagger \tilde{c}\right) ,$$
$$g = g_1 + i g_2. \tag{40}$$

The ensuing gap in the anticrossing is $\hbar 2|g| = \hbar 2\sqrt{g_1^2 + g_2^2}$.

Supplementary equations (35) - (40) constitute our final result and we pause to discuss their physical significance. The $\phi$ dependence of $g_1$ [$g_2$] is governed by $I_{\rm x,ip}(\phi)$ and $I_{\rm y,ip}(\phi)$ [$I_{\rm z,oop}(\phi)$], which in turn depends on the ellipticity of the magnon mode and the spatial overlap between the phonon and magnon wavefunctions, and by the factors $\sin(2\phi)$ and $\cos(2\phi)$ [$\cos(\phi)$] coming directly from the form of magneto-elastic coupling, Supplementary Eq. (33). The relative importance of $g_1$ and $g_2$ is additionally controlled by the factors $t_{\rm x,y,z}$ which parametrize the relative magnitude of the different displacements in the phonon mode.

### D: Exemplary coupling strengths calculated employing the model

The theoretical model described above was employed to calculate the coupling strength as a function of different combinations of the displacement weighting factors ($t_{\rm x,y,z}$) and the SAW decay length ($z_{\rm d}$). The magnetic mode profiles were obtained from TetraX [11, 12] simulations conducted using the experimentally determined anticrossing field ($B_{\rm ac}$) and a fixed wave vector equal to that of the SAW. In Supplementary Fig. 10a), the three cases representing pure displacement components are shown. These cases represent scenarios where only one displacement component is considered ($t_i = 1$, with the other two set to zero). The resulting angular dependence of the coupling strength exhibits maxima at different angles depending on the dominant displacement component. Notably, the maximum coupling occurs at 0° only when the y-displacement component is dominant ($t_{\rm y} = 1$). Panel b) illustrates the coupling strength calculated using the combination $t_{\rm y} = 0.89$ and $t_{\rm z} = 0.46$. With varying SAW decay length, the coupling strength changes in magnitude. If employing a less symmetric decay function for the SAW is assumed, instead of a purely exponential one, it allows for modifications to the symmetry of the coupling strength's angular dependence. Lastly, panel c) shows different combinations of $t_{\rm x,y,z}$, changing the ratio between $t_{\rm x}$ and $t_{\rm z}$. The parameters for the calculations are detailed in the figure caption. The specific parameters used for the theoretical curve presented in main text Fig. 3g) are $t_{\rm y} = 0.89$, $t_{\rm z} = 0.46$, $t_{\rm x} = 0$ with a decay length of $z_{\rm d} = 1.465\,\mu$m.

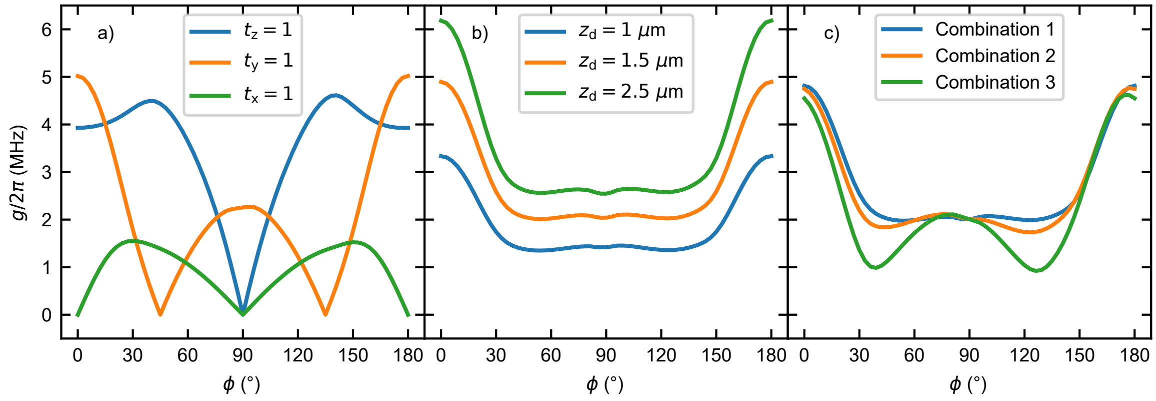


**Supplementary Fig.** 10: a) Theory curves for $z_{\rm d} = 1.465\,\mu$m, where only displacements in one direction are taking into account. This is achieved by setting $t_{\rm x,y,z}$ to one. b) Theory curves for $t_{\rm x} = 0$, $t_{\rm y} = 0.89$, $t_{\rm z} = 0.46$ with varying $z_{\rm d}$. c) Theory curves for $z_{\rm d} = 1.465\,\mu$m, with varying displacement $u_{\rm x,z}$ contributions. Combination 1: $t_{\rm x} = 0$, $t_{\rm y} = 0.89$, $t_{\rm z} = 0.46$. Combination 2: $t_{\rm x} = 0.2$, $t_{\rm y} = 0.89$, $t_{\rm z} = 0.41$. Combination 3: $t_{\rm x} = 0.4$, $t_{\rm y} = 0.89$, $t_{\rm z} = 0.22$.

## Supplementary Note 8: Sample fabrication

The device was fabricated on a 1.98 µm thick YIG layer grown on a 500 µm GGG substrate. A 976 nm thick piezoelectric ZnO layer was deposited onto the YIG via radio frequency magnetron sputtering, following a presputter cleaning of the YIG surface.

Microstructures were defined using a double-layer PMMA resist (PMMA 200K 4% AR-P 649.04, PMMA 950K 2% AR-P 679.02) patterned by electron beam lithography (EBL) at 20 kV. A conductive polymer (Espacer 300Z) was used to mitigate charging during EBL. The resist was developed in a 7:3 isopropanol to water solution. An oxygen plasma etch was used to remove residual PMMA in the exposed areas.

The fabrication process involved three EBL and lift-off steps using electron beam evaporation:

1. Alignment marks and a dose test were fabricated using a 5 nm Ti / 80 nm Au stack.
2. IDTs and SAW mirror structures were patterned using a 5 nm Ti / 30 nm Au stack in a single writing step for precise alignment.
3. Contact pads were fabricated using a 5 nm Ti / 150 nm Au stack with a thicker PMMA resist double layer (PMMA 600K 4% AR-P 669.04, PMMA 950K 2% AR-P 679.0) to ensure a sufficient undercut for lift-off.

The fabrication was performed at the nano structuring center at RPTU in Kaiserslautern, with ZnO sputtering carried out in the Clarendon Laboratory in Oxford.

## Supplementary References


[1] Sebastian, T., Schultheiss, K., Obry, B., Hillebrands, B. & Schultheiss, H. Micro-focused brillouin light scattering: imaging spin waves at the nanoscale. *Front. Phys.* **3** (2015).

[2] Geilen, M. *et al.* Interference of co-propagating rayleigh and sezawa waves observed with micro-focused brillouin light scattering spectroscopy. *APL* **117**, 213501 (2020).

[3] Ryburn, F. *et al.* Generation of gigahertz-frequency surface acoustic waves in $Y_3Fe_5O_{12}$/ZnO heterostructures. *Phys. Rev. Appl.* **23**, 034062 (2025).

[4] Manenti, R. *et al.* Surface acoustic wave resonators in the quantum regime. *Phys. Rev. B* **93** (2016).

[5] Schuetz, M. J. A. *et al.* Universal quantum transducers based on surface acoustic waves. *Phys. Rev. X* **5**, 031031 (2015).

[6] Maier-Flaig, H. *et al.* Note: Derivative divide, a method for the analysis of broadband ferromagnetic resonance in the frequency domain. *Rev. Sci. Instrum.* **89** (2018).

[7] Kittel, C. On the theory of ferromagnetic resonance absorption. *Phys. Rev.* **73**, 155–161 (1948).

[8] Kunz, Y. *et al.* Efficient spin-wave excitation by surface acoustic waves in ultra-low damping yig/zno-heterostructures (2025). 2503.11203.

[9] Weiler, M. Magnetization dynamics and spin torques in exchange–coupled spin systems (2019). Habilitation Thesis.

[10] Cohen-Tannoudji, C., Diu, B. & Laloë, F. *Quantum mechanics. Volume 1: Basic concepts, tools, and applications* (Wiley-VCH Verlag GmbH & Co. KGaA, Weinheim, 2020), second edition edn.

[11] Körber, L. *et al.* TetraX: Finite-Element Micromagnetic-Modeling Package (2022).

[12] Körber, L., Quasebarth, G., Otto, A. & Kákay, A. Finite-element dynamic-matrix approach for spin-wave dispersions in magnonic waveguides with arbitrary cross section. *AIP Adv.* **11**, 095006 (2021).

[13] Komiyama, H. *et al.* Quantitative evaluation method for magnetoelastic coupling between surface acoustic waves and spin waves using electrical and optical measurements (2024).

[14] Kittel, C. *Quantum Theory of Solids* (Wiley, 1963).

[15] Kamra, A. & Belzig, W. Magnon-mediated spin current noise in ferromagnet | nonmagnetic conductor hybrids. *Phys. Rev. B* **94**, 014419 (2016).

[16] Mills, D. Quantum theory of spin waves in finite samples. *J. Magn. Magn. Mater* **306**, 16–23 (2006).

[17] Zhang, X., Bauer, G. E. & Yu, T. Unidirectional pumping of phonons by magnetization dynamics. *Phys. Rev. Lett.* **125**, 077203 (2020).

[18] Comstock, R. Magnetoelastic coupling constants of the ferrites and garnets. *Proc. IEEE* **53**, 1508–1517 (1965).
